# Supplementary material for: Tracking Objects as Pixel-wise Distributions
Source: arXiv:2207.05518 source file (2022-07-15)
Supplement: Supplementary file 1 [file supplementary.tex]

\begin{figure}[th]
\centering
\includegraphics[width=\textwidth]{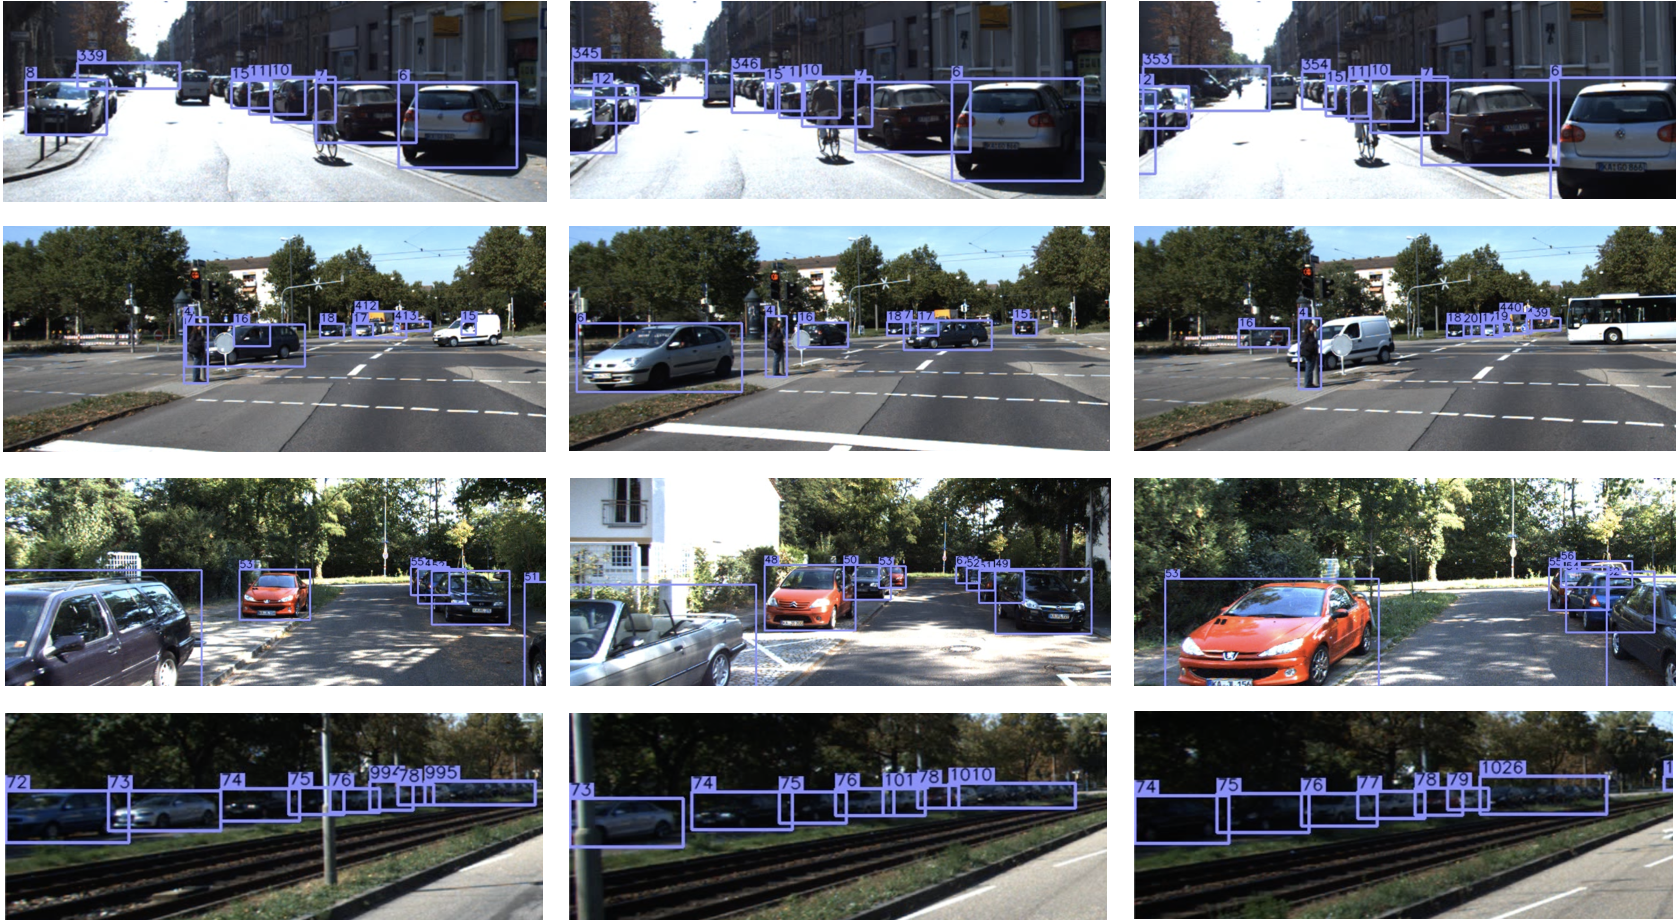}
\caption{Visualization of tracking results of P3AFormer on \texttt{KITTI-val}.}
\label{fig:kitti_visualization}
\vspace{-6mm}
\end{figure}

\section{Extended related work}
This section mentions some related work not included in the main text due to spatial constraints.

\subsection{Pixel-wise tracking}
Bibby et al.~\cite{pixelPosteriors} uses pixel-wise posterior to model object relationships across frames, and their work is not a deep learning method. After that, an unpublished work from Song et al.~\cite{song2017pixel} proposes to adopt pixel-wise information in single-object tracking, which relies on segmentation annotations. A recent benchmark STEP~\cite{stepTrackEveryPixel,fong2022panoptic} requires segment and track every pixel, which is different from standard MOT settings.

\subsection{Understanding vision transformers}
Several recent findings of vision transformers inspire the design of the P3AFormer. First, local inductive biases can improve the training of vision transformer~\cite{vitunderstand,SwinTransformer}, which supports the mask attention~\cite{mask2former}. Second, the training of vision transformers can be unstable due to negative Hessian eigenvalues~\cite{vitunderstand}. Heavy data augmentations~\cite{vitunderstand,vit} can mitigate this effect. Moreover, pixel-wise techniques may further smooth the loss landscapes~\cite{vitunderstand}, which motivates our training scheme.

\section{Methodology details}
We provide more details of the methodology parts in this section.
\subsection{Pixel-wise similarity function}
During pixel-wise propagation, we adopt a pixel-wise similarity function proposed by~\cite{flowGuidedFeatureAggregation}. Given two feature maps $\mathbf{P}_{l}^{(t)}$ and $\mathbf{P}_{l}^{(t-1)->(t)}$, the pixel-wise similarity of each location $p$ is computed as:
\begin{equation}
    w^{(t-1)->(t)}(p)=\exp \left(\frac{\mathbf{P}_{l}^{(t)}(p) \cdot \mathbf{P}_{l}^{(t-1)->(t)}(p)}{\left|\mathbf{P}_{l}^{(t)}(p)\right|\left|\mathbf{P}_{l}^{(t-1)->(t)}(p)\right|}\right).
\end{equation}

\begin{algorithm}[H]
\SetAlgoLined
 \textbf{Input}: tracks, center heatmaps confidence scores, bounding boxes\;
 \textbf{Output:} updated tracks\;
 Predict new locations of tracks via Kalman Filter\;
 Match the tracks with the predicted heatmaps via the Hungarian algorithm\;
 \For{all unmatched objects}{initialize a new track for it if its confidence is larger than the threshold $\eta_s$\;}
 Remove a track if it's dead for $n_k$ frames\;
 \caption{Pixel-wise association at timestep $t$.}
\label{alg:association}
\end{algorithm}

\subsection{Pixel-wise Association Algorithm}
Here we sketch the pixel-wise association in Algorithm~\ref{alg:association}. This algorithm depicts the same procedure as \textbf{Fig.3.} of the main text.

\section{Experimental details}
\subsection{Training process.} The input image is of shape $1440 \times 800$ for MOT17/MOT20 and $1280\times 384$ for KITTI. Following~\cite{yolox,bytetrack}, we use data augmentation, such as Mosaic~\cite{yolov4} and Mixup~\cite{mixup,automixup}. We use AdamW~\cite{adaw} with an initial learning rate of $6\times 10^{-5}$. We adopt the poly learning rate schedule~\cite{poly} with weight decay $1\times 10^{-4}$. The full training procedure lasts for 200 epochs. The P3AFormer models are all trained with eight Tesla V100 GPUs. The specific configurations of the losses are provided in the supplementary. The run-time analysis of different models is provided in the supplementary.
\subsection{Loss configurations}
The weight for the cross-entropy loss is 0.1, the focal loss is 0.5, and we use 1.0 for the size loss.
\subsection{Ablation studies}
We specify the details of the ablated models in this subsection.
\subsubsection{Vanilla Model} When we remove all the pixel-wise techniques from P3AFormer, the model is reduced to a vanilla deformable DETR~\cite{deformabledetr} and the association strategy is purely based on the detected bounding boxes.
\subsubsection{Pro.} We add feature propagation to the vanilla model, which means the model consumes two frames as input via the backbones and uses the pixel-wise feature propagation to align the pixel-level feature embeddings. The pixel-level embeddings are sent to the DETR decoder~\cite{DETR} to get the final predictions. The rest parts are the same as the vanilla model.
\subsubsection{Pre.} We leverage our proposed pixel decoder and the object decoder to get the object centers and sizes. Those predictions are directly sent to the tracker, and the tracking is purely based on the bounding boxes.
\subsubsection{Pre.+Ass.} We output the center heatmaps via the Pre. Model and track objects via the pixel-wise association algorithm.
\subsubsection{Pro.+Pre.} We adopt multi-frame input in the Pre. model and track objects based on bounding boxes.
\subsubsection{Pro.+Pre.+Ass.} This is the full P3AFormer model.

\setlength{\tabcolsep}{4pt}
\begin{table}
\begin{center}
\caption{Running time of different models on the MOT17 dataset.}
\label{tab:running_time}
\begin{tabular}{l|c}
\toprule
Model & Time (ms) \\ \midrule
TransCenter~\cite{Transcenter} & 112.4 \\
MOTR~\cite{MOTR} & 132.3 \\
P3AFormer (ours) & 108.2 \\ \bottomrule
\end{tabular}
\end{center}
\vspace{-8mm}
\end{table}
\setlength{\tabcolsep}{1.4pt}

\setlength{\tabcolsep}{4pt}
\begin{table}[ht]
\begin{center}
\caption{Validating the effectiveness of the matching threshold $\eta_m$ on \texttt{MOT17-val}.}
\label{tab:hyper_m}
\begin{tabular}{l|cc}
\toprule
$\eta_m$ & MOTA $\uparrow$ & IDF1 $\uparrow$\\ \midrule
0.75  & 76.3 & 75.1 \\
\textbf{0.65}  & 78.4 & 76.0 \\
0.55  & 76.6 & 75.7 \\
\bottomrule
\end{tabular}
\end{center}
\begin{center}
\caption{Validating the effectiveness of the track initialization threshold $\eta_s$ on \texttt{MOT17-val}.}
\label{tab:hyper_s}
\begin{tabular}{l|cc}
\toprule
$\eta_s$ & MOTA $\uparrow$ & IDF1 $\uparrow$\\ \midrule
0.90  & 77.8 & 72.9 \\
\textbf{0.80}  & 78.4 & 76.0 \\
0.70  & 74.2 & 73.6 \\
\bottomrule
\end{tabular}
\end{center}
\begin{center}
\caption{Validating the effectiveness of the kill-dead threshold $n_k$ on \texttt{MOT17-val}.}
\label{tab:nk}
\begin{tabular}{l|cc}
\toprule
$n_k$ & MOTA $\uparrow$ & IDF1 $\uparrow$\\ \midrule
40 & 75.1 & 72.6 \\
\textbf{30} & 78.4 & 76.0 \\
20  & 73.4 & 76.4 \\
\bottomrule
\end{tabular}
\end{center}
\vspace{-8mm}
\end{table}
\subsection{Generalization experiments}
We give more details of the generalization experiments. Our implementation is based on their official released code. The vanilla Tractor model predicts the temporal realignment of bounding boxes and uses a re-id network to enhance the association of the objects.

\subsubsection{+Pro.} We adopt the pixel-wise feature propagation to align the feature maps of consecutive frames extracted by the backbone before sending them into heads.

\subsubsection{+Pro.+Pre.} We change the shape of heads to output pixel-wise center heatmaps and sizes. The rest parts are the same as Tractor.

\subsubsection{+Pro.+Pre.+Ass.} We use our proposed pixel-wise association algorithm to associate the pixel-wise predictions from the modified Tracktor model. Note that the reID and motion models are not used in this setting.

\subsection{Run-time analysis of tracking models}
We evaluate the running time of different models: TransCenter~\cite{Transcenter}, MOTR~\cite{MOTR} and ours. The results are presented in Table~\ref{tab:running_time}. The running time is averaged for each frame. We observe that our pixel-wise techniques do not increase the overall running time (because our pixel-wise association techniques can be implemented efficiently via matrix operations). Although the transformer-based approaches are generally slower than the highly optimized detectors~\cite{bytetrack}, we believe transformers can become more efficient~\cite{reformer} in the future.

\subsection{Ablation studies on hyperparameters}
We change various hyperparameters in pixel-wise association and the results are presented in Table~\ref{tab:hyper_m}, Table~\ref{tab:hyper_s} and Table~\ref{tab:nk}. We find that the P3AFormer can work well under a variety of hyper-parameters.

\subsection{Visualizations}
We provide more visualizations on the KITTI dataset in Figure~\ref{fig:kitti_visualization}. We found that P3AFormer can track small objects of different classes on the KITTI dataset.
